# Supplementary material for: Pd/Pt embedded CN monolayer as efficient catalysts for CO oxidation
Source: arXiv:1909.11922 source file (2019-09-26)
Supplement: Supplementary file 1 [file Supporting_information.pdf]

# Supporting Information

## Pd/Pt embedded CN monolayer as efficient catalysts for CO oxidation

Yong-Chao Rao and Xiang-Mei Duan*

Department of Physics, Ningbo University, Ningbo-315211, P.R. China,

E-mail: duanxiangmei@nbu.edu.cn

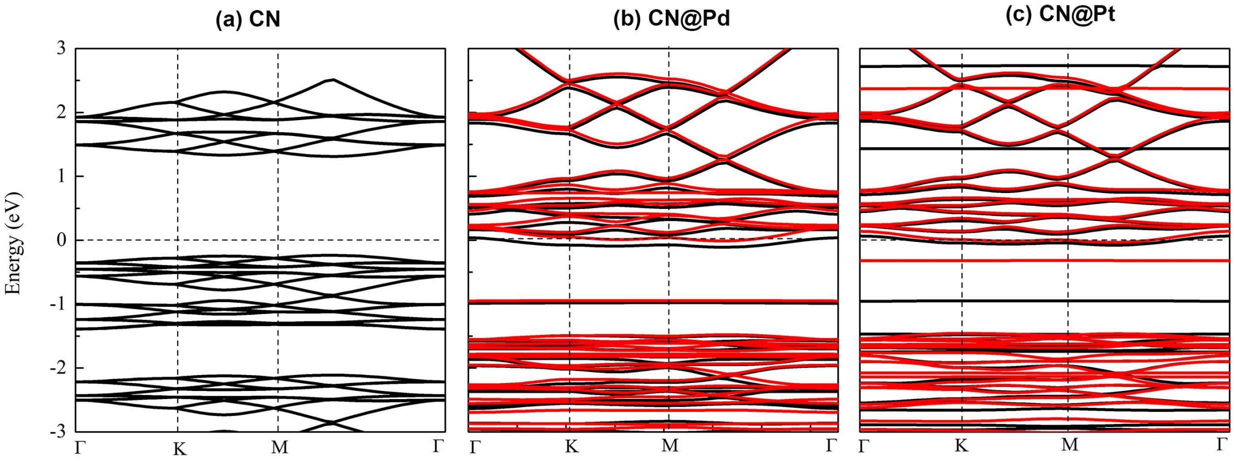


Fig. S1 The energy band structures based on PBE functional. The black and red lines represent the spin-up and spin-down bands.

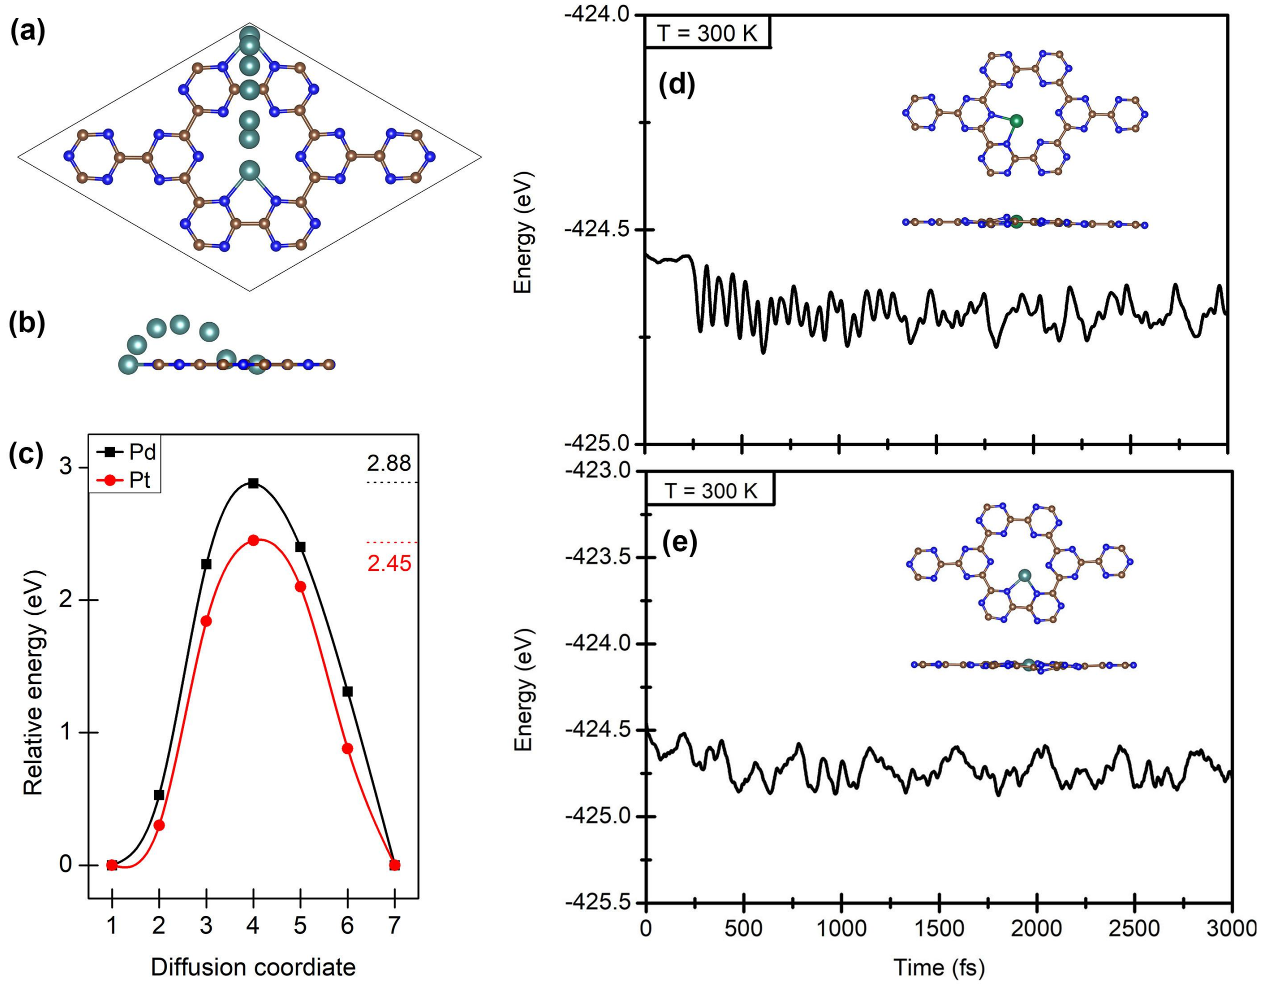


Fig. S2 The top (a) and side (b) view of migration pathway and corresponding minimum diffusion barriers (c) for Pd (black) and Pt (red) shifting between two nearby hexagonal holes on CN sheet. The total energy as a function of time for Pd@CN (d) and Pt@CN (e) at 300 K.

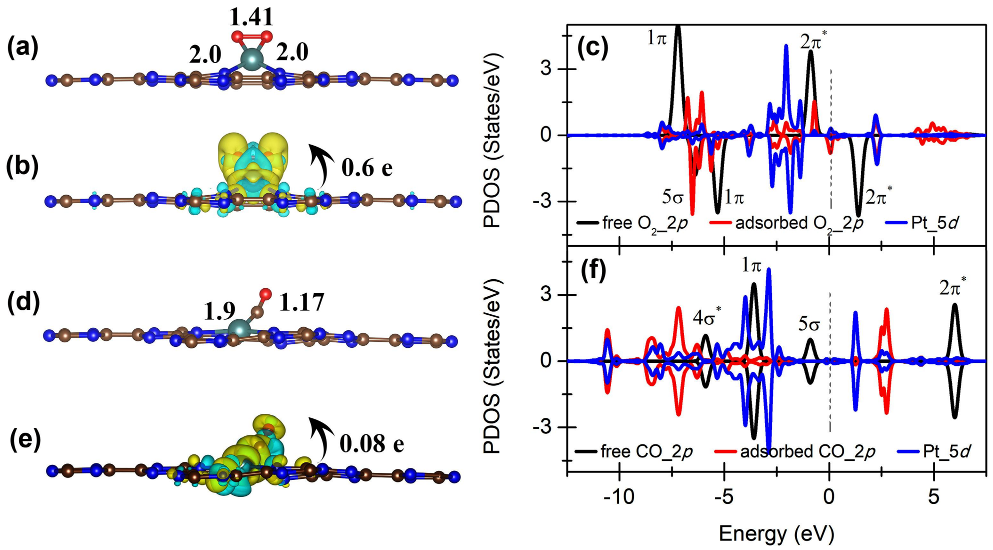


Fig. S3 The side views of optimized structures and corresponding charge density difference plots with an iso-surface value of 0.002 $e$/bohr$^3$, as well as spin-polarized PDOS for $O_2$ [(a), (b), (c)] and CO adsorption [(d), (e), (f)] on Pt@CN, respectively. The blue and yellow iso-surfaces represent the electron depletion and accumulation, and the Fermi level is set at zero,

| | O | $CO_2$ | $O_2$+CO | CO+CO |
|---|---|---|---|---|
| CN-Pd | 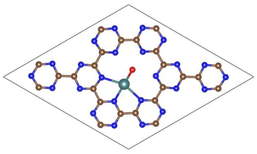 | 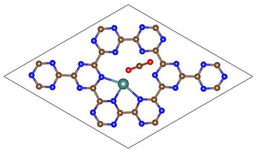 | 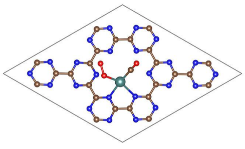 | 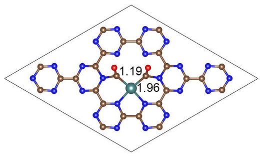  |
| | 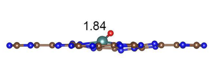  | 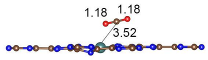  | 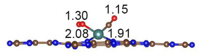  | 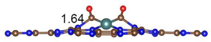  |
| $E_a$ | -4.20 | -0.11 | -1.25 | -2.37 |
| CN-Pt | 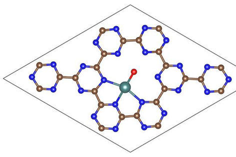 | 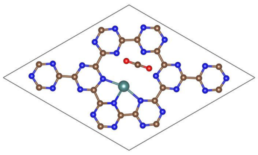 | 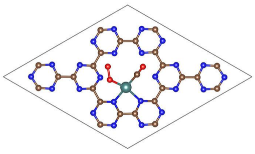 | 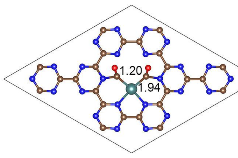  |
| | 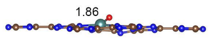  | 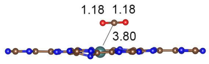  | 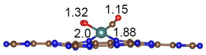  | 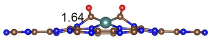  |
| $E_a$ | -5.21 | -0.48 | -2.56 | -4.09 |

Fig. S4 The top and side views of optimized structures for adsorption of atomic O, $CO_2$, $O_2$+CO, and CO+CO on Pd/Pt@CN, respectively, as well as the respective adsorption energy ($E_a$).
